# Supplementary material for: Tuning Confidence Bound for Stochastic Bandits with Bandit Distance
Source: arXiv:2110.02690 source file (2021-10-06)
Supplement: Supplementary file 3 [file appendix.tex]

\section{Regret Curves}
\label{apn:regret_curve}

\begin{figure}[H]
	\centering
	\scalebox{0.28}{
		\input{plots/pgf_link/regrets.pgf}
	}
	\caption{Regret of different policies as a function of time (log scale) in each environment.}
	\label{fig:exp}
\end{figure}


\section{More Bandit Distances}
\label{apn:more_d}

We experiment the following two additional distances:

\begin{description}
	\item [UCB-then-Commit]
	$$
	d_t(i, j) = \begin{dcases}
	0 & N_i(t) \leq \floor{1 / \gamma} \\
	1 & N_i(t) > \floor{1 / \gamma}
	\end{dcases}
	$$
	\item [UCB-DT($\mu$ margin)] $d_t(i, j) = \left(|\hat{\mu}_i(t) -
	\hat{\mu}_j(t)| - m \right) ^{1 / \floor{\gamma N_i(t)}}$
\end{description}

We name the first strategy as UCB-then-Commit, similar to Explore-then-Commit as
in \citep{even2006action, garivier2016explore,garivier2019explore}. This strategy
is simple and can be used to verify whether a proper bandit distance can help to
spend exploration budget on bandits close to the optimal one. For the second
strategy, we subtract a margin term $m$ from the mean distance. We summarize their cumulated
regrets in table \ref{tab:more_dist}.



\begin{table}[h]
	\centering
	\begin{tabular}{lrrrr}
		\hline
		Experiment    & UCB     & UCB-DT($\mu$) & UCB-then-Commit &        
		UCB-DT($\mu$ margin)                                               \\
		\hline
		B5            & 251.28  & 70.95         & 76.11           & 73.49  \\
		B20           & 939.99  & 383.82        & 436.36          & 415.68 \\
		B(0.02, 0.01) & 249.17  & 21.6          & 58              & 243.04 \\
		B(0.9, 0.88)  & 119.91  & 19.19         & 105.7           & 110.01 \\
		N5            & 142.21  & 83.65         & 185.44          & 108.11 \\
		N20           & 1014.27 & 640.52        & 778.72          & 628.14 \\
		\hline
	\end{tabular}
	\vspace*{2pt}
	\caption{Regret of UCB and UCB-DT on more distances in each environment.
		$\gamma$ is set to 0.02 in all experiments, $m$ is set to 0.05.}
	\label{tab:more_dist}
\end{table}


Comparing UCB-DT($\mu$) and UCB-then-Commit, it is clear to see that spending
exploration budget around the neighbor of the optimal bandit is helpful. It is
also interesting to see that UCB-then-Commit generally outperforms UCB by a
large margin, which indicates a benefit of under exploration as in Sec.
\ref{sec:under_exploration}. UCB-DT($\mu$ margin) is slightly better than
UCB-DT($\mu$) in N20, probably because of the margin term which keeps the
exploitation more conservative when the mean estimation is not robust enough.



\section{Formulation of Standard UCB}

Recall the \citep[Chapter~7]{lattimore2020bandit}, UCB is derived from
Hoeffding's inequality on sum of subgaussian variables. Let $X_{1}, X_{2}, \ldots, X_{n}$ be independent and L1-subgaussian
random variables with zero mean and $\hat{\mu}=\sum_{t=1}^{n} X_{t} / n$, then


\begin{equation}
	\mathbb{P}(\hat{\mu} \geq \varepsilon) \leq \exp \left(-n \varepsilon^{2} / 2\right)
	\label{eq:concen}
\end{equation}

Replacing $\exp \left(-n \varepsilon^{2} / 2\right)$ with $\delta$ then we get


\begin{equation}
	\mathbb{P}\left(|\hat{\mu}| \geq \sqrt{\frac{2}{n} \log \left(\frac{1}{\delta}\right)} \right) \leq \delta
	\label{eq:ucb_dawn}
\end{equation}

If we use $1/t$ for $\delta$, we arrive to the formulation of UCB


\section{Optimal Exploration and Exploration Bargain Point}
\label{apn:ebp_more}

From our analysis, we gain a deeper understanding of why UCB is an "optimistic"
policy. Furthermore, we can set the derivative of the lower bound in Eq.
\ref{eq:gain_bargain} on $N_2$ to 0 and solve for the optimal bound, which
represents the optimal exploration-exploitation trade-off point. We
calculate result in Eq. \ref{eq:N2star} with \citep{Mathematica}.


\begin{equation}
	\begin{split}
		&\left\{N_{2}^* \to \frac{\mu _1^2 T-2 \mu _2 \mu _1 T+\mu _2^2 T-16 W_{c_1}\left(\frac{1}{2} e^{\frac{\mu
			_1^2 T}{16}-\frac{1}{8} \mu _2 \mu _1 T+\frac{\mu _2^2 T}{16}+1}\right)+16}{2
		\left(\mu _2-\mu _1\right){}^2} \bigg| c_1 \in \mathbb{Z} \right\} \\
		& \text{where }  W \text{ denotes the Lambert $W$ function}
	\end{split}
	\label{eq:N2star}
\end{equation}

The exact solution of $N_{bargain}$ cannot be solved analytically and we only solve them
numerically in Fig. \ref{fig:example_ebp}.  The difficulty lies in the Eq.
\ref{eq:transend}, which is transcendental and has no closed formula for $N_2$.


\begin{equation}
	\begin{split}
		0 & = e^{-\frac{1}{16} \Delta ^2 _2 N_2} \left(2 N_2-T\right) - N_2+\frac{8 \log
			(T)}{\Delta _2^2} \\
		\text{the} & \text{ solution of this equation for $N_2$ is \textit{Exploration Bargain Point}}
	\end{split}
	\label{eq:transend}
\end{equation}



There are many hidden intrigues behind our new analysis tool. For example,
Eq.~\ref{eq:N2star} represents a set of local optimal points for cumulated
rewards, what is the relationship between them and which one has practical
relevance. Moreover, like the connection between transcendental equation and
exploration exploitation trade-off, the super-logarithm function $W$ in Eq.
\ref{eq:N2star} and the $\overline{\log}$ in \citep{lattimore2018refining}, and
the logical link between $N_{full}$ and worst case regret bound, are very
interesting to explore.
